# Supplementary material for: GS-ROR$^2$: Bidirectional-guided 3DGS and SDF for Reflective Object Relighting and Reconstruction
Source: arXiv:2406.18544 source file (2026-06-02)
Supplement: Supplementary file 1 [file supp.pdf]

# Supplementary Material – GS-ROR: 3D Gaussian Splatting for Reflective Object Relighting via SDF Priors

## 1 LOSS DETAILS

We introduce the definition and weights of losses we used in the main paper. The color loss is defined as in 3DGS [Kerbl et al. 2023]

$$L_c = \lambda \|C_{gs} - C_{gt}\|_1 + (1 - \lambda)(1 - \text{SSIM}(C_{gs}, C_{gt})), \quad (1)$$

where  $C_{gs}$  is the rendered color from Gaussians and  $C_{gt}$  is the ground truth color. The coefficient  $\lambda$  is set to 0.8. The supervision  $L_{nd}$  from normal is defined as

$$L_{nd} = \|\hat{\mathbf{n}} - \mathbf{n}\|^2, \quad (2)$$

where  $\hat{\mathbf{n}}, \mathbf{n}$  are the normal from depth and the normal from Gaussians, respectively. Our normal formulation follows Gaussian Shader, which combines the shortest axis and a learnable residual [Jiang et al. 2024] as

$$\mathbf{n} = u + n_\delta, \quad (3)$$

where  $u$  is the shortest axis and  $n_\delta$  is the residual term. To prevent the residual from dominating the normal direction, we add a penalty to it:

$$L_{\delta_n} = \|n_\delta\|^2. \quad (4)$$

The smoothness loss for BRDF parameters (*i.e.*, albedo  $\mathbf{a}$ , roughness  $\mathbf{r}$ , metallicity  $\mathbf{m}$ ) is defined as

$$L_{sm} = \|\nabla f\| \exp^{-\|\nabla C_{gt}\|}, (f \in \{\mathbf{a}, \mathbf{r}, \mathbf{m}\}) \quad (5)$$

where  $\nabla$  is the gradient operator and  $C_{gt}$  is the color of ground-truth image. The mask loss is the binary cross entropy between predicted and ground-truth masks.

In the first phase, we set the corresponding weights  $\lambda_{[\cdot]}$  as  $\lambda_{nd} = 0.2$ ,  $\lambda_{sm} = 1e^{-2}$ ,  $\lambda_m = 0.2$ ,  $\lambda_{\delta n} = 1e^{-3}$ . In the second phase, the loss weights are set as  $\lambda_{gs2sdf} = 0.5$ ,  $\lambda_{eik} = 0.1$ ,  $\lambda_{hes} = 5e^{-4}$ ,  $\lambda_{tv} = 0.1$ . In third phase, the loss weights are set as  $\lambda_{sdf2gs} = 0.25$ .

## 2 SPLIT-SUM APPROXIMATION

A typical rendering equation needs to compute an integral on the upper hemisphere involving incident light, view direction, normal, and BRDF (Bidirectional Reflectance Distribution Function):

$$c(\omega_o) = \int_{\Omega} L_i(\omega_i) f(\omega_i, \omega_o) (\omega_i \cdot \mathbf{n}) d\omega_i, \quad (6)$$

where  $L_i(\omega_i)$  denotes the light from incident direction  $\omega_i$ ,  $f(\omega_i, \omega_o)$  is the BRDF with respect to the incident direction  $\omega_i$  and outgoing direction  $\omega_o$ , and  $\mathbf{n}$  denotes the surface normal. In practice, the Disney Principled BRDF [Burley and Studios 2012] is the most widely used BRDF, consisting of a diffuse lobe and a specular lobe

$$f(\omega_i, \omega_o) = \underbrace{(1 - \mathbf{m}) \frac{\mathbf{a}}{\pi}}_{\text{diffuse}} + \underbrace{\frac{DFG}{4(\omega_i \cdot \mathbf{n})(\omega_o \cdot \mathbf{n})}}_{\text{specular}}, \quad (7)$$

where  $D$  is the normal distribution function,  $F$  is the Fresnel term,  $G$  is the geometry term,  $\mathbf{a}$  is the albedo, and  $\mathbf{m}$  is the metallicity. However, the integral is expensive to evaluate, and the split-sum

Author's address:

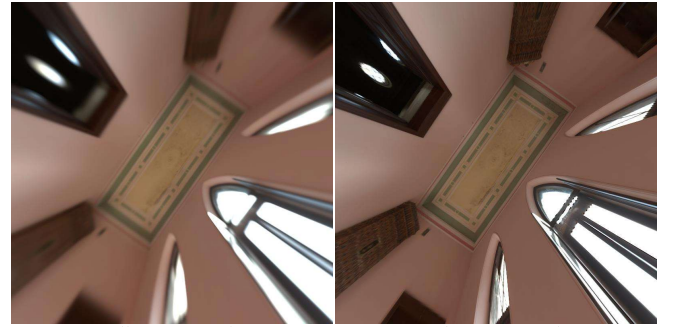

Split-sum Results

Path Trace Results

Fig. 1. The comparison between the result using Cycle path-tracing renderer in Blender and the one using split-sum approximation in DiffRast. The split-sum result is blurry when the roughness of the surface is very small.

technique [Karis and Games 2013] is an alternative widely used in real-time rendering. The specular term is approximated as

$$c_{\text{specular}} \approx L_{\text{specular}} \cdot ((1 - \mathbf{m}) \times 0.04 + \mathbf{m} \times \mathbf{a}) \times F_1 + F_2, \quad (8)$$

where  $F_1, F_2$  are two scalars from a pre-computed table. The diffuse term is computed as

$$c_{\text{diffuse}} = \frac{\mathbf{a}(1 - \mathbf{m})}{\pi} \cdot L_{\text{diffuse}}. \quad (9)$$

$L_{\text{diffuse}}$  and  $L_{\text{specular}}$  can be directed queried for a pre-filtered environment map or neural light representations. The rendered color  $c(\omega_o)$  is computed as  $c(\omega_o) = c_{\text{diffuse}} + c_{\text{specular}}$ .

However, as illustrated in the main paper, when the roughness is very small, the split-sum approximation leads to blurry results. We render a mirror-like plane in Blender using Cycle path-tracing renderer and in the DiffRast [Laine et al. 2020] using the split-sum approximation. The comparison is in Fig. 1, and we can see the split-sum result is blurry.

## 3 LIGHT MODELING

Considering the efficiency of the light query, we use a simple differential environment map and do not model the indirect illumination and occlusion. The environment light is in the cube map format, whose resolution is  $6 \times 512 \times 512$ .

## 4 MORE RESULTS

In this section, we present more results and comparisons.

### 4.1 Glossy Blender Dataset

We present the LPIPS [Zhang et al. 2018] of relighting images on the Glossy Blender dataset in Tab. 1 and Tab. 2. Our method outperforms Gaussian-based methods along with some NeRF-based ones and is competitive with the current SOTA method.

## 4.2 Shiny Blender dataset

We show the NVS and relighting results on the Shiny Blender dataset [Verbin et al. 2022]. The quantitative comparison of NVS results are in Tab. 3 and Tab. 4. Our method outperforms the existing Gaussian-based methods on most scenes. However, our method fails in the “coffee” scene, for the deferred pipeline assumes an opaque surface, and the liquid in the “coffee” does not meet the assumption. As illustrated in Fig. 3, our method can provide sharper highlights and more realistic NVS results. We present the relighting result in Fig. 4. Our method provides photo-realistic relighting results, while other Gaussian-based methods fail to render highlights under novel light conditions. We show decomposed maps in Fig. 5, and our method can provide reasonable BRDF decomposition. Besides, we present a comparison of normal estimation in Fig. 6. Thanks to the SDF priors, our method can provide robust normal estimation, while the results of other Gaussian-based methods are overfitted or noisy.

## 4.3 TensolR synthetic dataset

We present the relighting quality of Gaussian-based methods on the TensolR synthetic dataset [Jin et al. 2023] in terms of LPIPS in Tab. 5 and the relighting visualization in Fig. 7. The relighting comparison with NeRF-based methods is in terms of PSNR, SSIM in Tab. 6 and LPIPS in Tab. 7. And the relighting visualization of NeRF-based methods is in Fig. 8. We also show the decomposed maps in

Fig. 9, and the comparison of normal with Gaussian-based methods in Fig. 10. These results of diffuse objects reveal that though our design focuses on reflective surfaces, it can benefit diffuse objects.

Table 3. NVS quality with Gaussian-based methods on Shiny Blender dataset in terms of PSNR $\uparrow$  and SSIM $\uparrow$ .

|         | GS-IR       | RelightGS          | GShader            | Ours               |
|---------|-------------|--------------------|--------------------|--------------------|
| Ball    | 18.30/.7584 | 21.39/.9047        | <u>30.40/.9623</u> | <b>35.50/.9849</b> |
| Car     | 25.30/.8867 | 26.59/.9267        | <u>28.39/.9388</u> | <b>30.52/.9638</b> |
| Coffee  | 30.72/.9463 | <b>32.57/.9710</b> | <u>30.79/.9690</u> | 29.64/.9568        |
| Helmet  | 25.08/.9018 | 26.95/.9469        | <u>28.78/.9549</u> | <b>32.62/.9738</b> |
| Teapot  | 38.21/.9900 | <u>43.86/.9963</u> | 43.35/.9957        | <b>43.88/.9964</b> |
| Toaster | 18.66/.7418 | 20.07/.8745        | <u>23.95/.9130</u> | <b>25.89/.9379</b> |
| Mean    | 26.05/.8708 | 28.57/.9367        | <u>30.94/.9556</u> | <b>33.01/.9689</b> |

Table 4. NVS quality with Gaussian-based methods on Shiny Blender dataset in terms of LPIPS $\downarrow$ .

|         | GS-IR  | RelightGS     | GShader       | Ours          |
|---------|--------|---------------|---------------|---------------|
| Ball    | 0.2966 | 0.2169        | <u>0.1358</u> | <b>0.0842</b> |
| Car     | 0.0849 | 0.0533        | <u>0.0477</u> | <b>0.0330</b> |
| Coffee  | 0.1125 | <b>0.0841</b> | <u>0.0853</u> | 0.1035        |
| Helmet  | 0.1618 | 0.1014        | <u>0.0866</u> | <b>0.0482</b> |
| Teapot  | 0.0222 | 0.0097        | <u>0.0108</u> | <b>0.0079</b> |
| Toaster | 0.2479 | 0.1523        | <u>0.1017</u> | <b>0.0859</b> |
| Mean    | 0.1543 | 0.1030        | <u>0.0779</u> | <b>0.0605</b> |

Table 1. Relighting quality with Gaussian-based methods on the Glossy Blender dataset in terms of LPIPS $\downarrow$ .

|        | GS-IR  | RelightGS | GShader       | Ours          |
|--------|--------|-----------|---------------|---------------|
| Angel  | 0.1901 | 0.1428    | <u>0.1181</u> | <b>0.0858</b> |
| Bell   | 0.5203 | 0.1431    | <u>0.1329</u> | <b>0.0795</b> |
| Cat    | 0.1591 | 0.1171    | <u>0.1114</u> | <b>0.0596</b> |
| Horse  | 0.1606 | 0.0866    | <u>0.0498</u> | <b>0.0356</b> |
| Luyu   | 0.1391 | 0.1094    | <u>0.1057</u> | <b>0.0672</b> |
| Potion | 0.2142 | 0.1614    | <u>0.1832</u> | <b>0.0937</b> |
| Tbell  | 0.3368 | 0.1970    | <u>0.1877</u> | <b>0.0953</b> |
| Teapot | 0.1716 | 0.1312    | <u>0.1194</u> | <b>0.0982</b> |
| Mean   | 0.2365 | 0.1361    | <u>0.1260</u> | <b>0.0769</b> |

Table 2. Relighting quality with NeRF-based methods on the Glossy Blender dataset in terms of LPIPS $\downarrow$ .

|        | TensoIR | MII    | TensoSDF      | NeRO          | Ours          |
|--------|---------|--------|---------------|---------------|---------------|
| Angel  | 0.2739  | 0.1404 | <u>0.0871</u> | 0.1923        | <b>0.0858</b> |
| Bell   | 0.2806  | 0.1534 | <u>0.0263</u> | <b>0.0189</b> | 0.0795        |
| Cat    | 0.2146  | 0.1429 | 0.0675        | <b>0.0455</b> | <u>0.0596</u> |
| Horse  | 0.2913  | 0.0713 | <b>0.0318</b> | 0.0410        | <u>0.0356</u> |
| Luyu   | 0.2463  | 0.1393 | 0.0807        | <u>0.0696</u> | <b>0.0672</b> |
| Potion | 0.2954  | 0.1747 | <u>0.0759</u> | <b>0.0623</b> | 0.0937        |
| Tbell  | 0.2786  | 0.1938 | <u>0.0543</u> | <b>0.0407</b> | 0.0953        |
| Teapot | 0.2030  | 0.1426 | <u>0.0485</u> | <b>0.0193</b> | 0.0982        |
| Mean   | 0.2605  | 0.1448 | <u>0.0590</u> | <b>0.0612</b> | 0.0769        |

Table 5. Relighting quality with Gaussian-based methods on the TensolR synthetic dataset in terms of LPIPS $\downarrow$ .

|         | GS-IR  | RelightGS     | GShader       | Ours          |
|---------|--------|---------------|---------------|---------------|
| Armada. | 0.0821 | <u>0.0593</u> | 0.0649        | <b>0.0482</b> |
| Ficus   | 0.0956 | 0.0366        | <b>0.0437</b> | <u>0.0439</u> |
| Hotdog  | 0.1408 | <u>0.0880</u> | 0.1275        | <b>0.0771</b> |
| Lego    | 0.1193 | <u>0.0902</u> | 0.1423        | <b>0.0724</b> |
| Mean    | 0.1095 | <u>0.0685</u> | 0.0946        | <b>0.0604</b> |

Table 6. Relighting quality with NeRF-based methods on the TensolR synthetic dataset in terms of PSNR $\uparrow$  and SSIM $\uparrow$ .

|         | MII         | NeRO               | TensoSDF           | TensoIR            | Ours               |
|---------|-------------|--------------------|--------------------|--------------------|--------------------|
| Armada. | 26.85/.9441 | 23.02/.9335        | 23.02/.9355        | <b>34.51/.9754</b> | <u>31.33/.9593</u> |
| Ficus   | 20.65/.9068 | <u>27.43/.9404</u> | <b>28.53/.9499</b> | 24.32/.9465        | 26.28/.9542        |
| Hotdog  | 22.65/.9011 | 20.45/.9262        | 20.47/.9241        | <b>27.92/.9324</b> | 25.21/.9307        |
| Lego    | 23.20/.8643 | 17.76/.8577        | 17.92/.8670        | <b>27.61/.9253</b> | 25.46/.9083        |
| Mean    | 23.34/.9041 | 22.17/.9145        | 22.48/.9191        | <b>28.59/.9449</b> | <u>27.07/.9381</u> |

Table 7. Relighting quality with NeRF-based methods on the TensorIR synthetic dataset in terms of LPIPS↓.

|        | MII    | NeRO   | TensoSDF      | TensorIR      | Ours          |
|--------|--------|--------|---------------|---------------|---------------|
| Armad. | 0.0692 | 0.0644 | 0.0578        | <b>0.0368</b> | <u>0.0483</u> |
| Ficus  | 0.0728 | 0.0677 | <u>0.0533</u> | 0.0543        | <b>0.0439</b> |
| Hotdog | 0.0893 | 0.0888 | <u>0.0906</u> | 0.0833        | <b>0.0771</b> |
| Lego   | 0.1715 | 0.1228 | 0.1088        | <b>0.0702</b> | <u>0.0723</u> |
| Mean   | 0.1007 | 0.0859 | 0.0776        | <u>0.0612</u> | <b>0.0604</b> |

## REFERENCES

- Brent Burley and Walt Disney Animation Studios. 2012. Physically-based shading at disney. In *SIGGRAPH*.
- Yingwenqi Jiang, Jiadong Tu, Yuan Liu, Xifeng Gao, Xiaoxiao Long, Wenping Wang, and Yuexin Ma. 2024. GaussianShader: 3D Gaussian Splatting with Shading Functions for Reflective Surfaces. In *CVPR*.
- Haian Jin, Isabella Liu, Peijia Xu, Xiaoshuai Zhang, Songfang Han, Sai Bi, Xiaowei Zhou, Zexiang Xu, and Hao Su. 2023. TensorIR: Tensorial Inverse Rendering. In *CVPR*.
- Brian Karis and Epic Games. 2013. Real shading in unreal engine 4. *Proc. Physically Based Shading Theory Practice* (2013).
- Bernhard Kerbl, Georgios Kopanas, Thomas Leimkühler, and George Drettakis. 2023. 3D Gaussian Splatting for Real-Time Radiance Field Rendering. *ACM TOG* (2023).
- Samuli Laine, Janne Hellsten, Tero Karras, Yeongho Seol, Jaakko Lehtinen, and Timo Aila. 2020. Modular Primitives for High-Performance Differentiable Rendering. *ACM TOG* (2020).
- Dor Verbin, Peter Hedman, Ben Mildenhall, Todd Zickler, Jonathan T. Barron, and Pratul P. Srinivasan. 2022. Ref-NeRF: Structured View-Dependent Appearance for Neural Radiance Fields. In *CVPR*.
- Richard Zhang, Phillip Isola, Alexei A Efros, Eli Shechtman, and Oliver Wang. 2018. The unreasonable effectiveness of deep features as a perceptual metric. In *CVPR*.

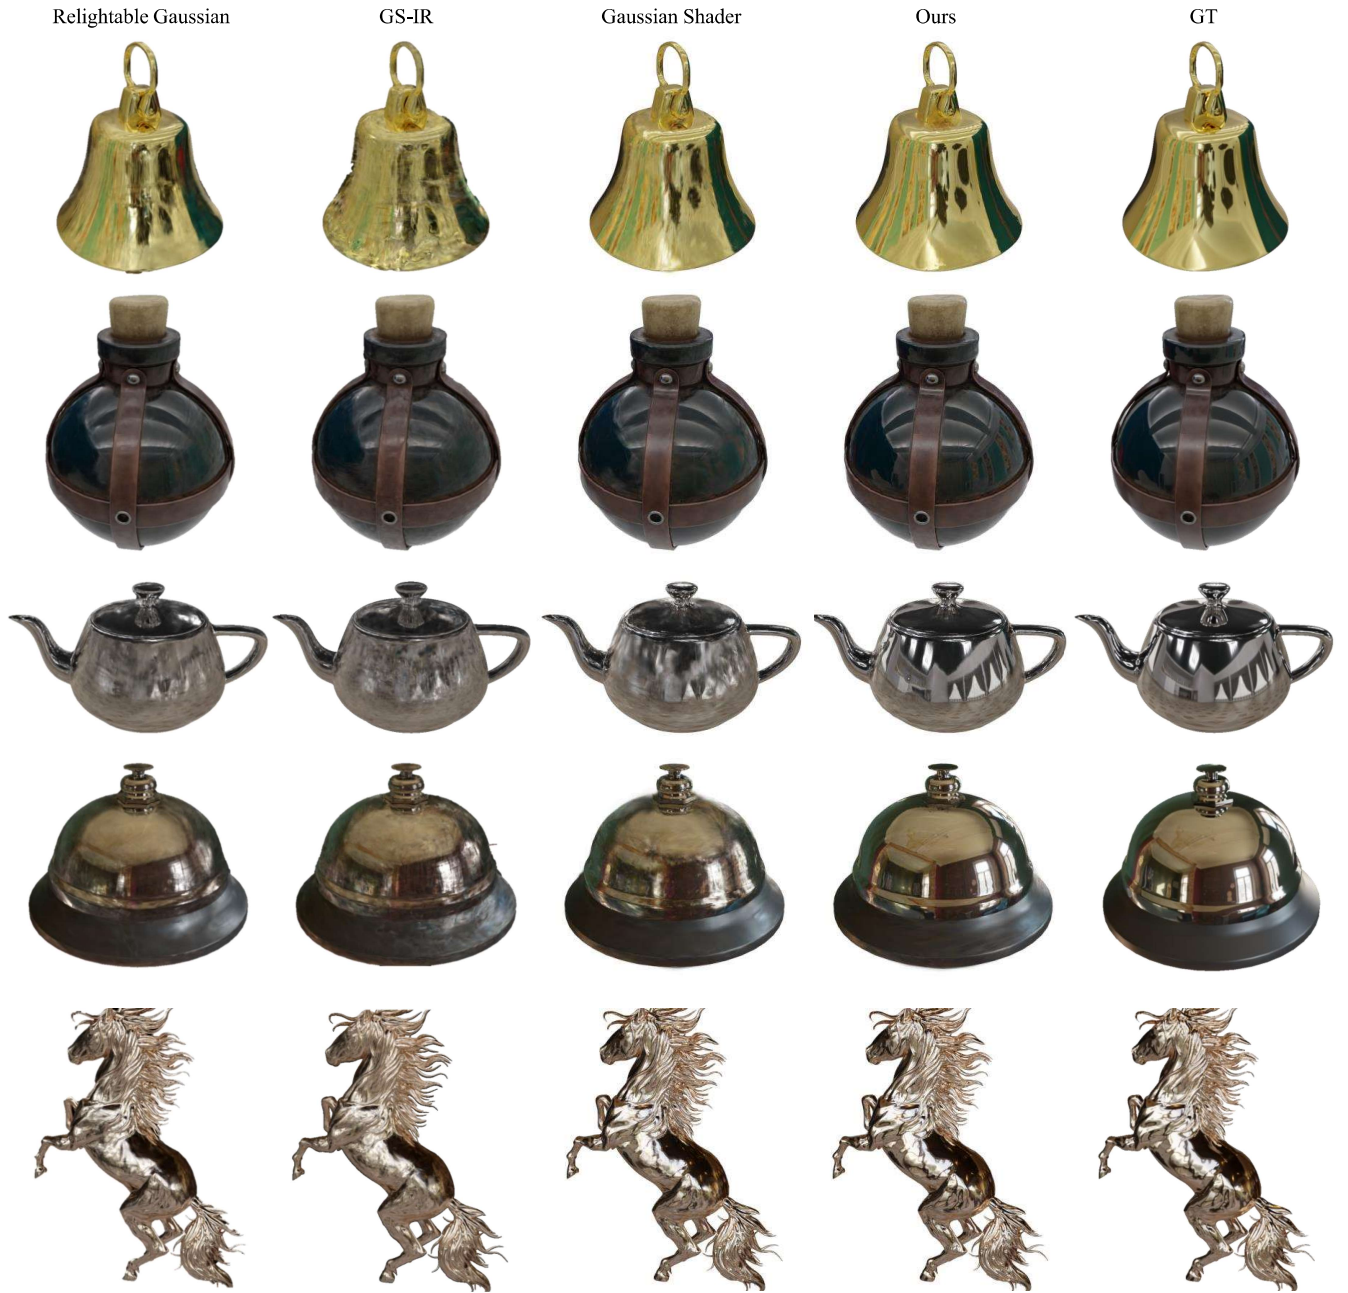

Fig. 2. NVS results on the Glossy dataset. Our method provides photo-realistic NVS results for reflective objects, while other Gaussian-based methods fail.

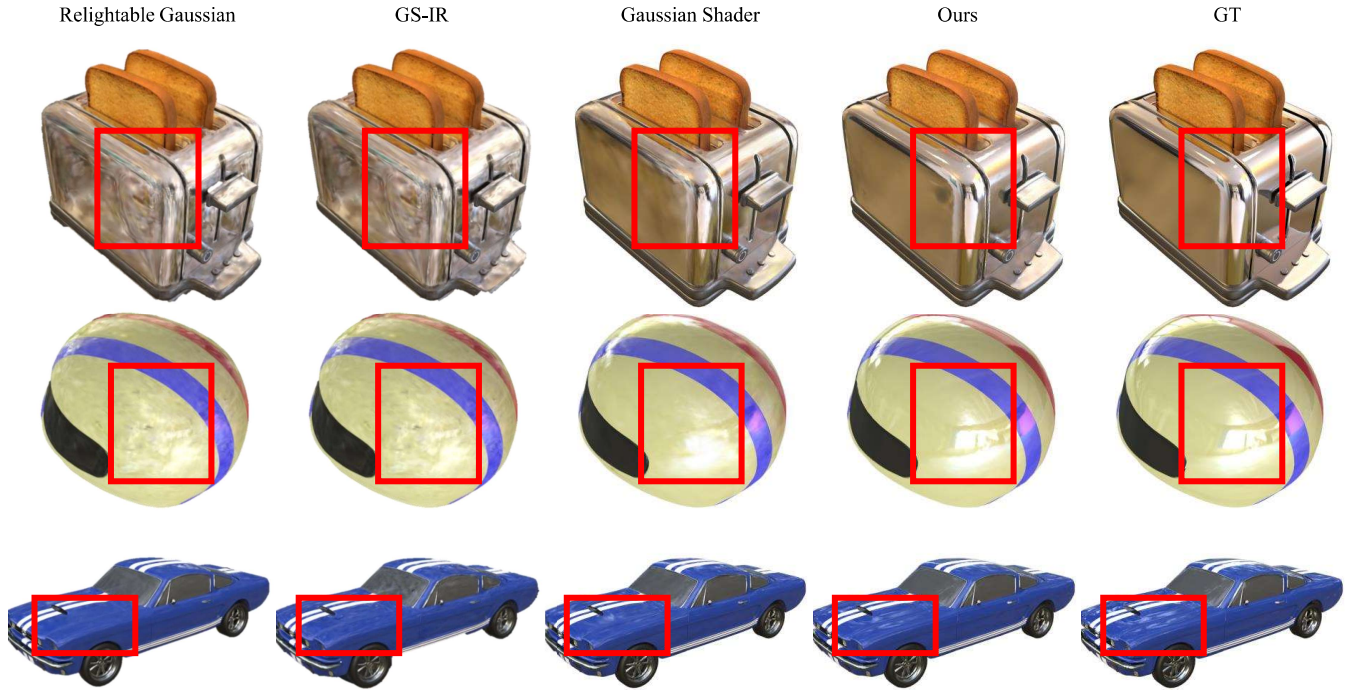

Fig. 3. NVS results of Gaussian-based methods on the Shiny Blender dataset. Our method preserves correct highlights, while others fail to render sharp highlights.

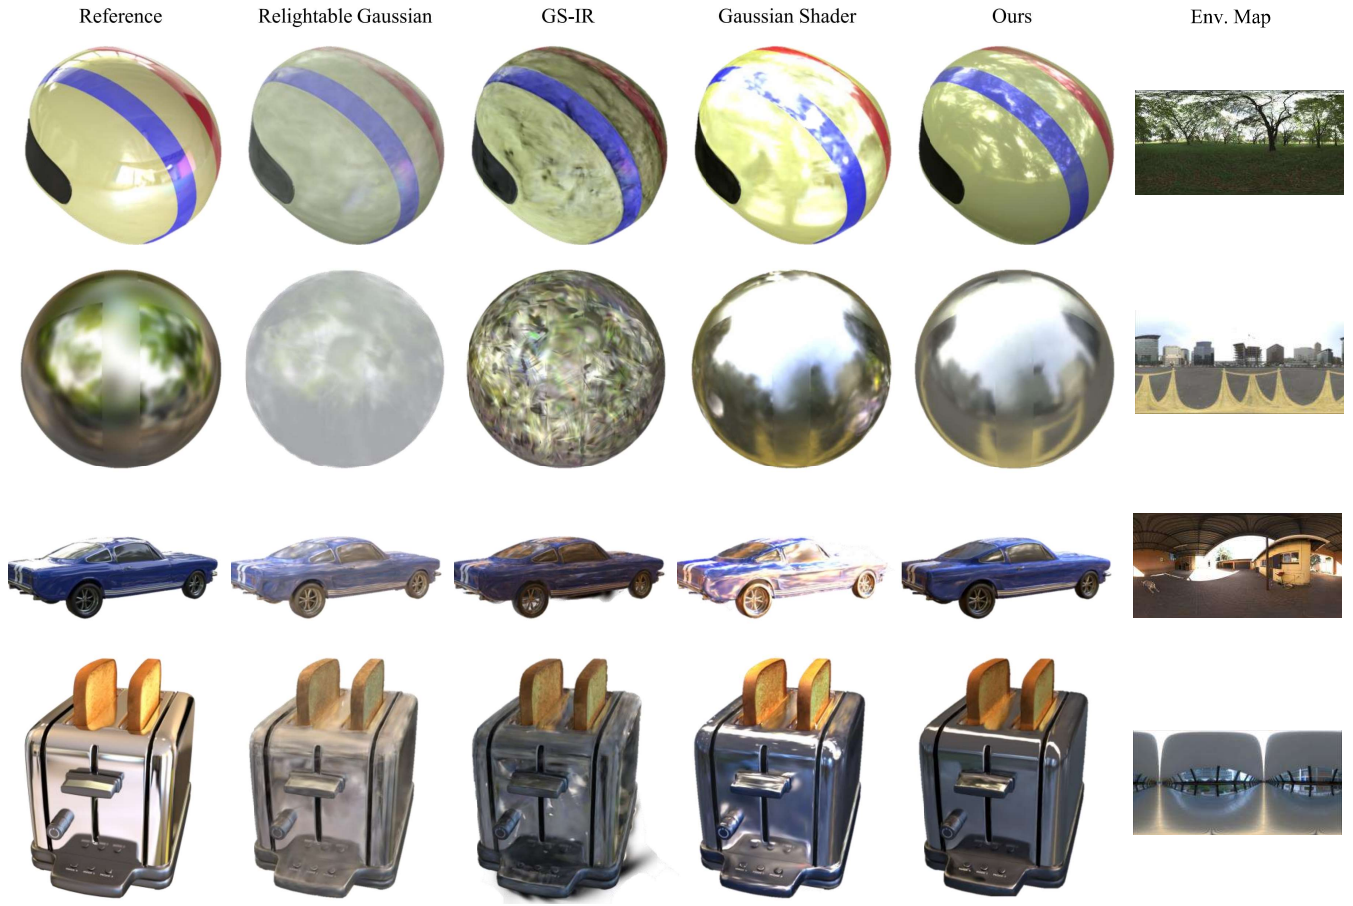

Fig. 4. Relighting results of Gaussian-based methods on the Shiny Blender dataset. Note that no relighting ground truth is available, so we only show the relighting examples. Our method can provide reasonable relighting results under diverse lighting conditions.

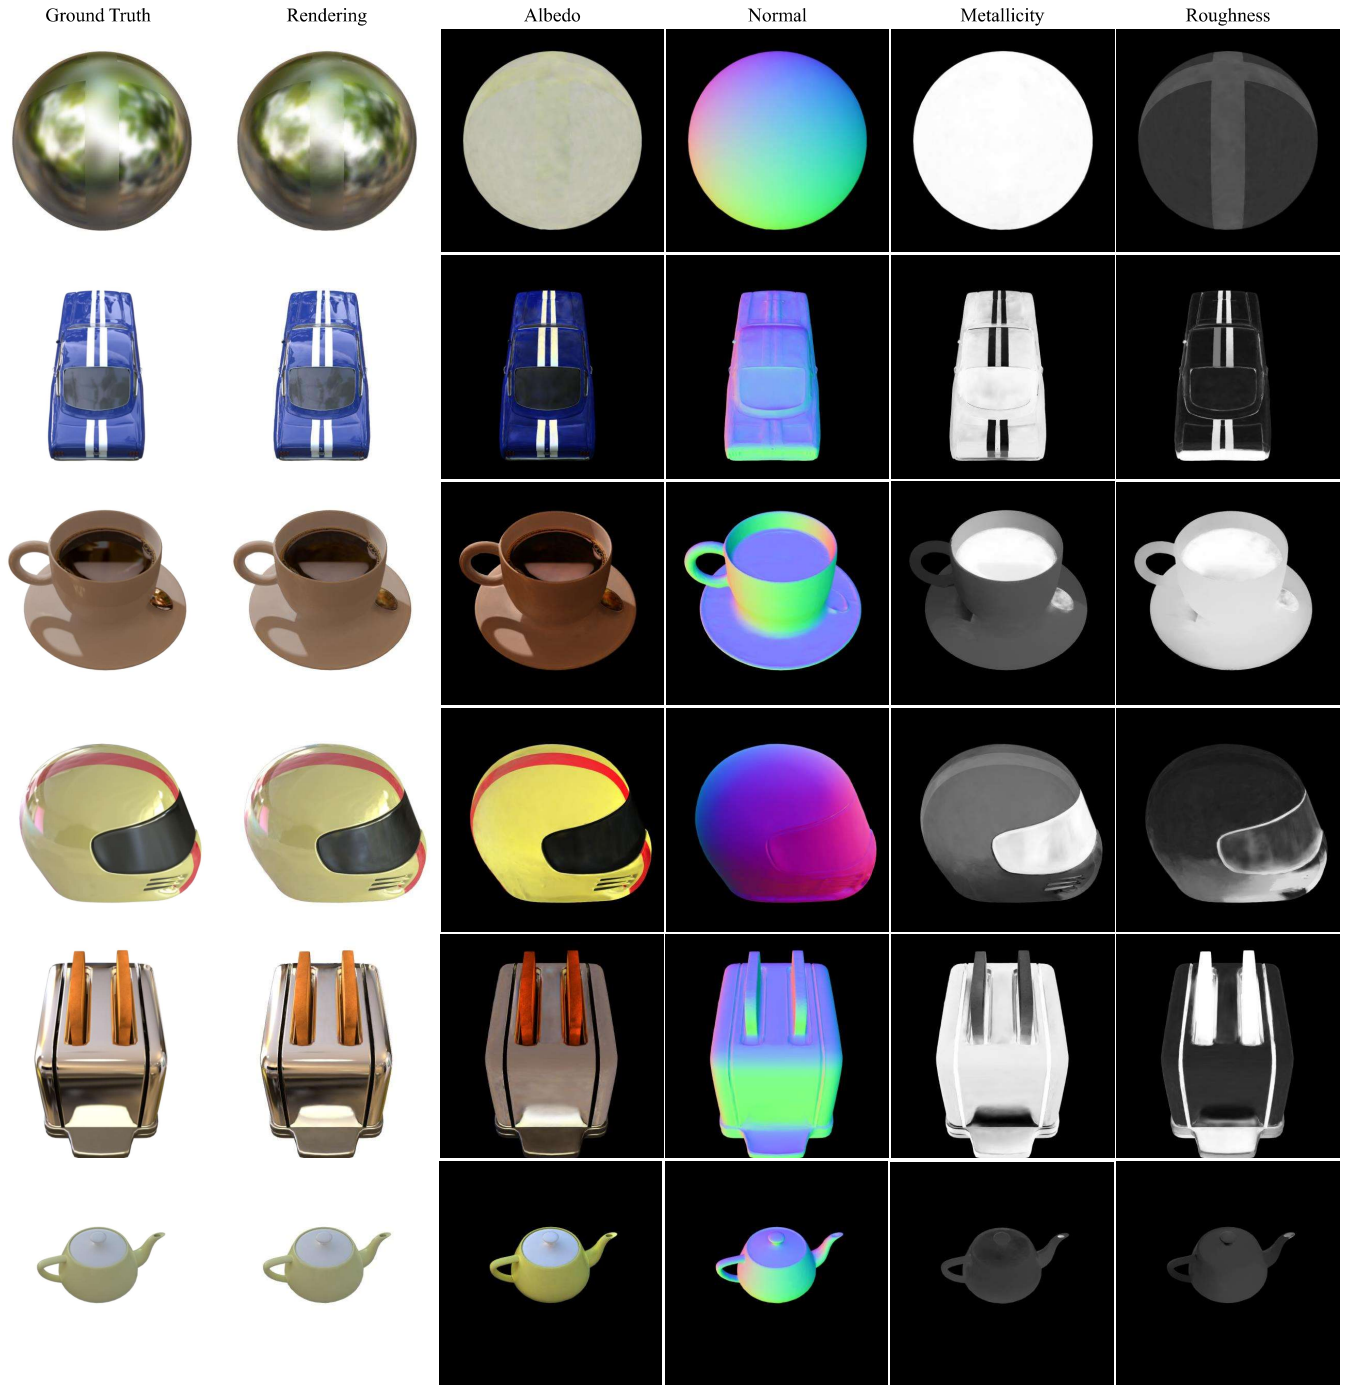

Fig. 5. Normal and BRDF decomposed maps on the Shiny Blender dataset. Our method provides robust normal estimation and reasonable BRDF decomposition.

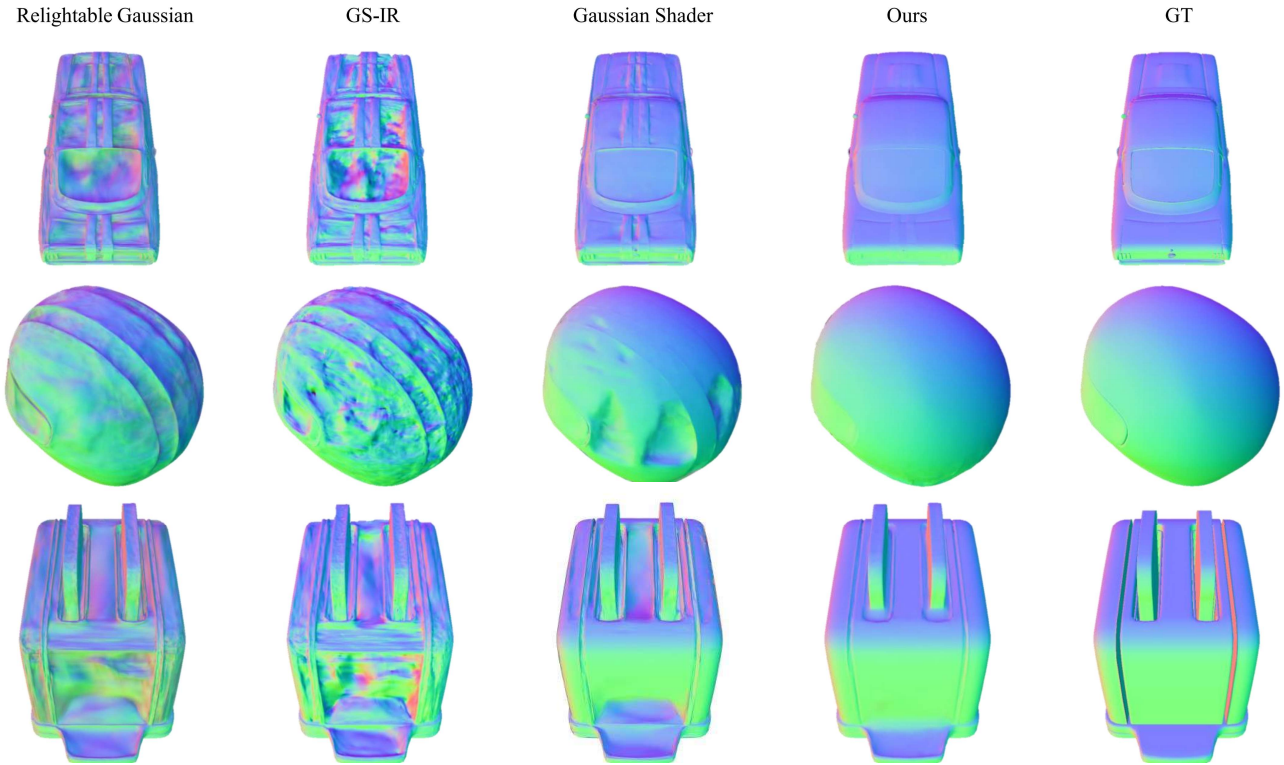

Fig. 6. Normal comparison with Gaussian-based methods on the Shiny Blender dataset. Our method provides robust normal estimation, while other results are noisy or overfitted.

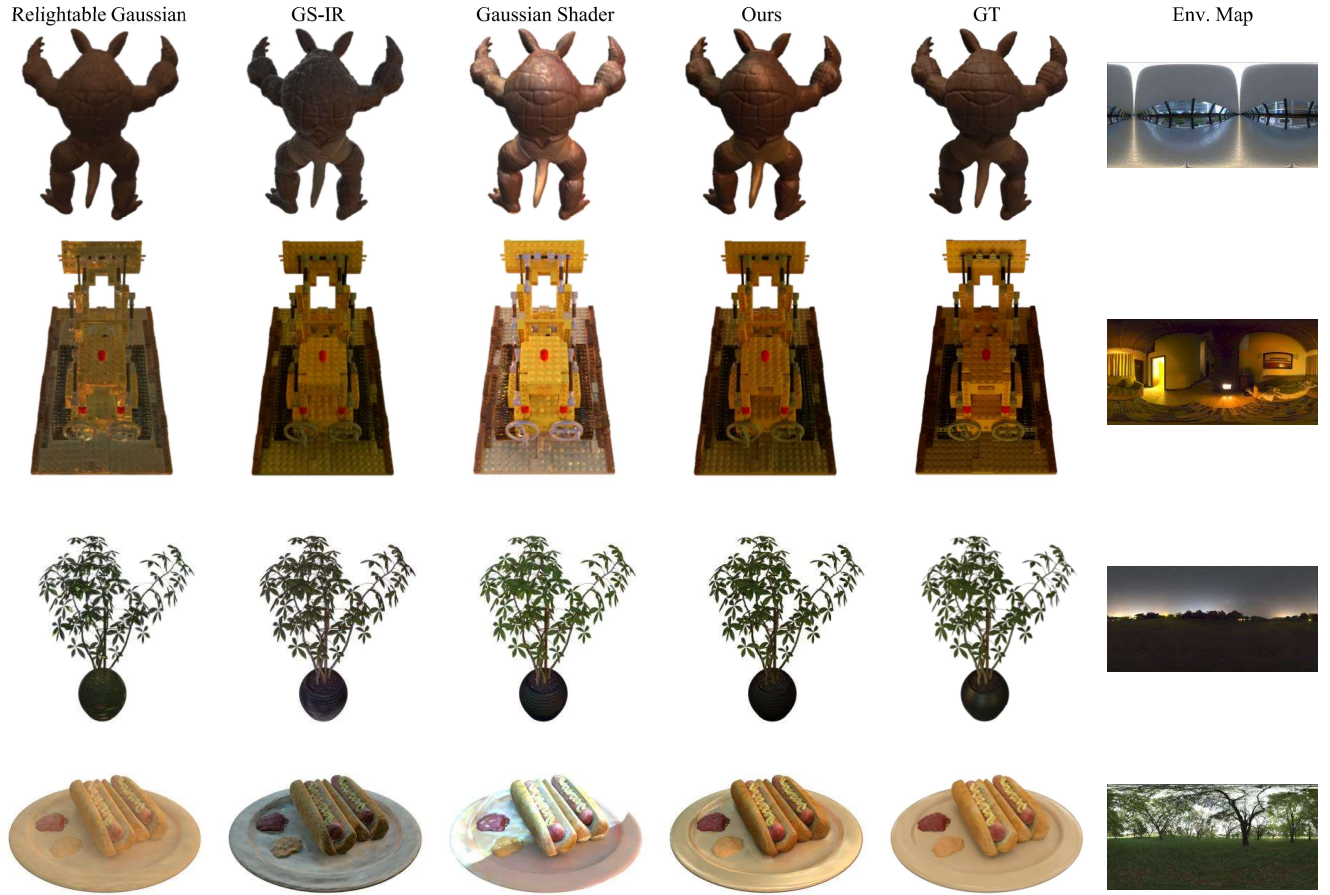

Fig. 7. Relighting results of Gaussian-based methods on the TensorIR synthetic dataset. Our method can also provide high-quality relighting results for diffuse objects and outperforms the existing Gaussian-based methods.

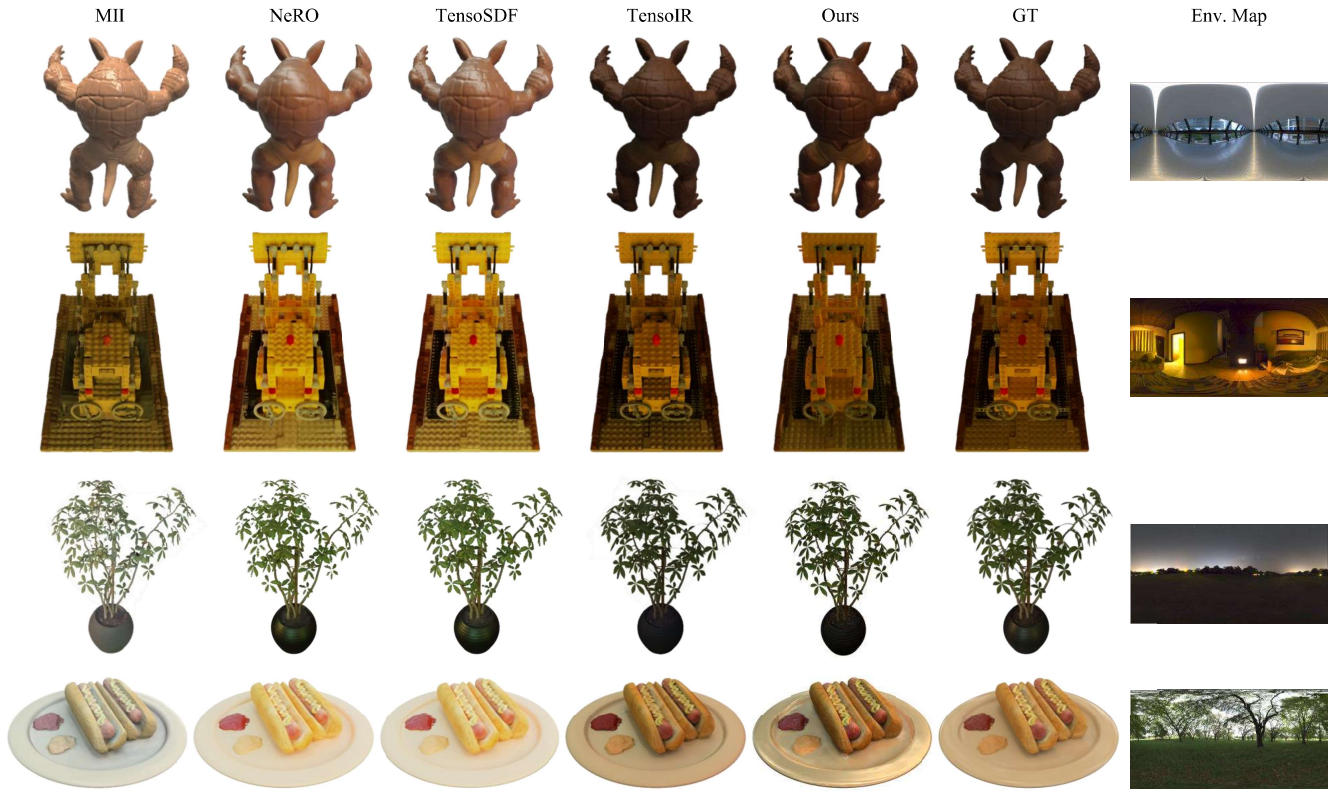

Fig. 8. Relighting results of NeRF-based methods on the TensorIR synthetic dataset. Our method can also provide high-quality relighting results for diffuse objects and outperforms most NeRF-based methods.

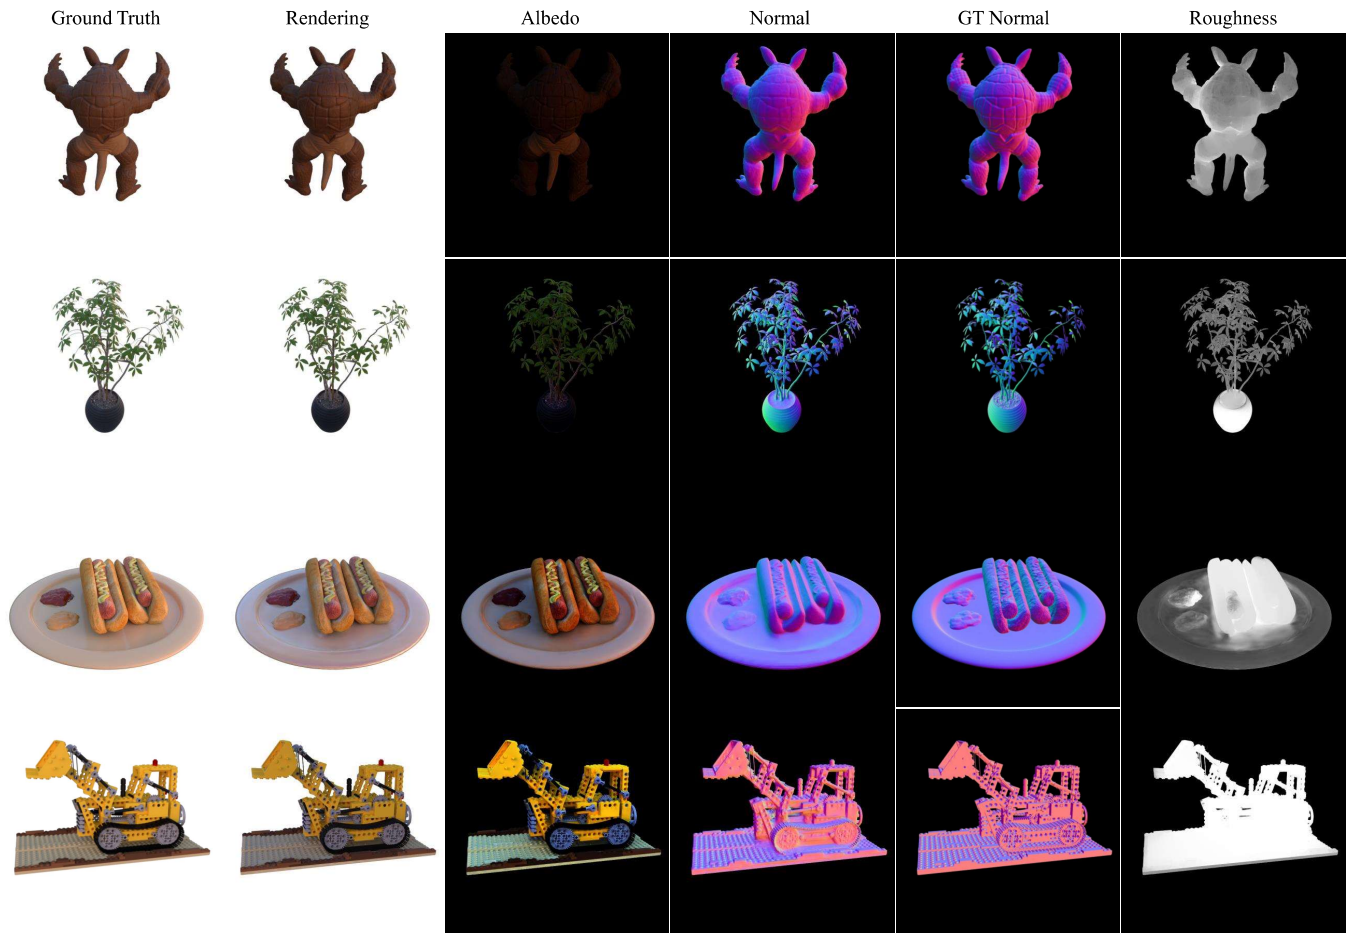

Fig. 9. Normal and BRDF decomposed maps of our method on the TensorIR synthetic dataset. Our method can also provide reasonable BRDF estimation for diffuse objects.

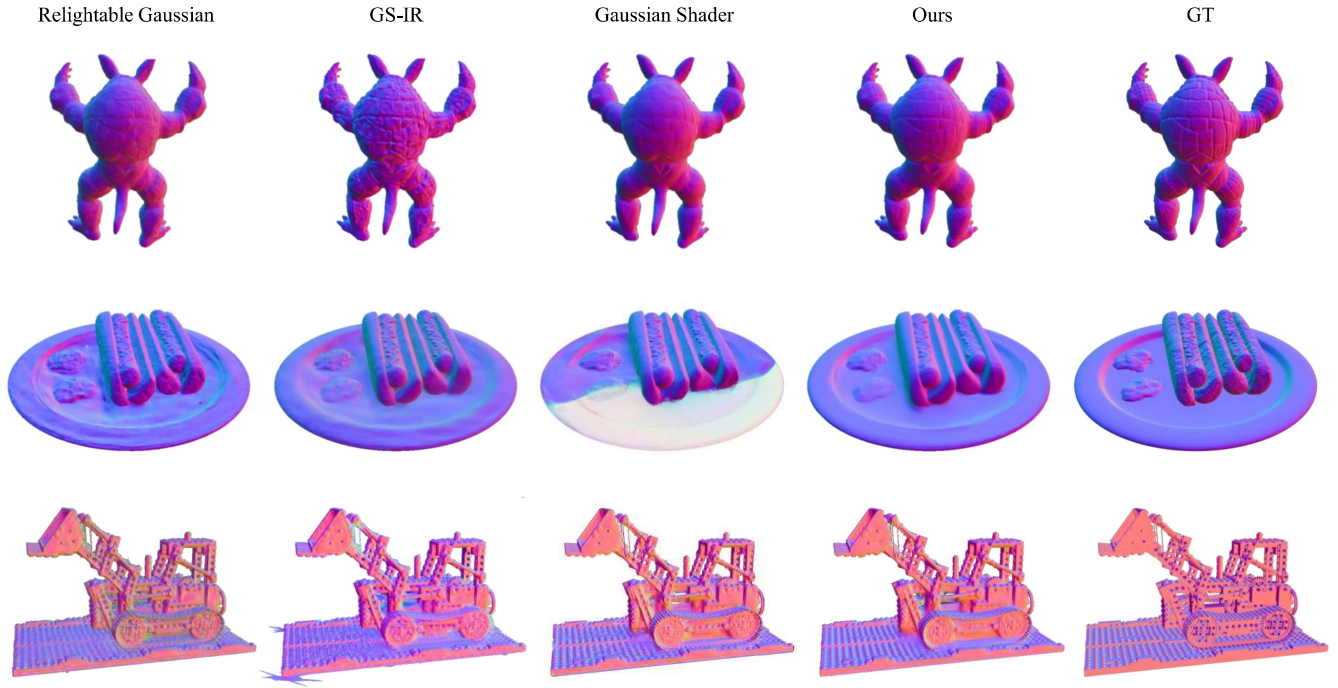

Fig. 10. Normal comparison with Gaussian-based methods on the TensorIR synthetic dataset. Our method can also provide robust normal estimation for diffuse objects.
